# Supplementary material for: JANUS: Benchmarking Commercial and Open-Source Cloud and Edge Platforms for Object and Anomaly Detection Workloads
Source: arXiv:2012.04880 source file (2020-12-09)
Supplement: Supplementary file 1 [file sec_appendix.tex]

\section{Appendix With Changes}

The details regarding the choice for the compute-intensive and compute-light workloads are now clearly explained. We selected the two types of IoT applications that are popular in a variety of real-world scenarios. We also added references related to the choices that explain usage in different scenarios and motivated the scenarios better. %We also expanded on the motivation for this work by citing which pieces of picking an infrastructure is non-trivial.

We picked Faster R-CNN over other popular open source object detection algorithms like SSD and YOLO and we explained the reasons why we chose it over the others, primarily because it is somewhat more accurate and is computationally more complex, making it more suitable for use in our compute-intensive scenario.

Since we used a Raspberry Pi as a physical edge device that is on the side of lightweight devices (in terms of compute resources), we wanted to include an emulated edge device with higher resources, especially as backends for running compute-intensive workloads. We added comments to explain how it could be comparable to more powerful edge devices, \eg the NVIDIA Jetson TX2. Our Docker emulation of more resourceful edge devices was leveraging the fact that different Docker instantiations can mimic differentially-resourced edge devices. We have provided references to back this claim.

We initially used the e2-medium instance in Google Compute, which is a shared-core instance, as opposed to c5.large and F2S\_v2, which are compute instances. We have thus switched the Google Compute instance to an e2-standard, which has dedicated cores. We did not notice much improvements in performance (on averaging over 5 runs, both e2-standard and e2-medium had a runtime of around 2.1s) , but the cost did change (\$0.06701 per hour for e2-standard vs. \$0.03351 per hour for e2-medium). This provided a more apples-to-apples comparison.

We also cleaned up on the writing and unified some terms like compute-intensive/compute-light workloads instead of heavyweight/lightweight workloads and data-heavy/data-light workloads. We have also unified ``dollar'' cost and ``\$'' cost. Furthermore, all figures have also been referred to.

% \begin{enumerate}
%     \item Unifying compute-light and compute-intensive
%     \item Included reasons for picking these two workloads in introduction
%     \item Included reasons for picking FRCNN over SSD and YOLO
%     \item Provided a small snippet to mention docker can represent higher powered edge devices like Nvidia Jetson
%     \item Changed e2-medium to e2-standard to use normal cores instead of shared cores. The numbers didn't change too much and averaged out to be about the same for object detection
%     \item Expanded on motivation by moving points from evaluation to introduction
% \end{enumerate}
